# Supplementary material for: Online Matching with Delays and Size-based Costs
Source: arXiv:2408.08658 source file (2024-08-16)
Supplement: Supplementary file 1 [file appendix.tex]

\section{Appedix for Upper Bound}

\begin{lem} \label{lmm:alpha_logk_loglogk}
   $2$ 以上の整数 $k$ に対して, $k \geq 3^3$ であれば $k = \alpha^\alpha$ となるような $\alpha \in \mathbb{R}$ を取る. $k < 3^3$ であれば, $\alpha = 3$ とする. このとき, $\alpha = \Theta(\log k / \log \log k)$ である.  
\end{lem}

\begin{proof}
がんばって証明する.
\end{proof}
